# Supplementary material for: The CoT Collection: Improving Zero-shot and Few-shot Learning of Language Models via Chain-of-Thought Fine-Tuning
Source: arXiv:2305.14045 source file (2023-10-14)
Supplement: Supplementary file 1 [file appendix.tex]

/section(
